# Supplementary material for: Uncoupled Bandit Learning towards Rationalizability: Benchmarks, Barriers, and Algorithms
Source: arXiv:2111.05486 source file (2023-12-23)
Supplement: Supplementary file 1 [file appendix-thm3Proof.tex]

\subsection{Preparations for the Proof}
We consider the DIR game in which the two agents are following Algorithm \ref{al:da} with non-increasing learning rate $\{\eta_t\}_{t=1}^{\infty}$ in a repeated game with the DIR game payoff matrix. In this proof, we shall always think of $c\geq 3K^2>K$, therefore the simplified DIR game matrix becomes the following  % given by Eq \eqref{eq:lowerboundinstance}.  
\begin{equation} 
\frac{1}{c } \times \begin{bmatrix} 
(1,1) & (1, -c) & (1, -c) & \cdots & (1, -c) \\
(2,1) & (2,2) & (2, -c) & \cdots  & (2, -c) \\
(-c, 1) & (3,2) & (3,3) & \cdots  & (3, -c) \\
\vdots & \vdots & \ddots & \ddots & \vdots \\
\vdots & \vdots & \vdots &  (K-1, K-1) & (K-1, -c) \\
(-c, 1) & (-c,2) & \cdots & (K, K-1) & (K, K) \\
\end{bmatrix}    
\end{equation}

Let $u_{A,i}(t), u_{B,i}(t), p_{A,i}(t), p_{B,i}(t)$ denote agent A and agent B's payoffs\footnote{For simplification of notation, we omit the $\tilde{}$ above $u$, but it is still the expected payoff of an action given opponent's strategy profile.} and probabilities of picking the $i$-th action at round $t$, respectively. We further let  $$y_{A,i}(t)=\sum_{s=1}^{t-1} u_{A,i}(s)\eta_s, \qquad y_{B,i}(t)=\sum_{s=1}^{t-1} u_{B,i}(s)\eta_s$$  be the $i$th arm's accumulated weights of agent A and agent B till round $t$. Then, according to the DA algorithm,  
$$(p_{A, 1}(t),\cdots,p_{A, K}(t))=Q(y_{A, 1}(t),\cdots,y_{A, K}(t)),$$ $$(p_{B, 1}(t),\cdots,p_{B, K}(t))=Q(y_{B, 1}(t),\cdots,y_{B, K}(t)).$$

The following is a simple yet useful fact regarding the mirror map induced by any symmetric regularizer. 
\begin{lemma}\label{lm:mono_Q}
For any mirror map $p = Q(y)$ with symmetric regularizer, if $y_i> y_j$, then $p_i\geq p_j$.
\end{lemma}
\begin{proof}
We prove by contradiction. Suppose for some $\y$ and $i, j$ where $y_i > y_j$, while $\p = Q(y)$ with $p_i < p_j$. By definition, $\p = Q(\y) =\arg\max_{x\in \Delta_K}\{\langle \y,\x \rangle-h(\x)\}$. However, consider the vector $\tilde{\p}= (p_1, \dots, p_j, \dots, p_i, \dots, p_{K})$. By construction, $\tilde{\p} \in \Delta_K$ and $h(\tilde{\p}) = h(\p) $. By rearrangement inequality, we have $\tilde{p}_i y_j + \tilde{p}_j y_j  = p_j y_i + p_i y_j > p_i y_j + p_j y_j $ such that $\langle \y,\tilde{\p} \rangle-h(\tilde{\p}) > \langle \y,\p \rangle-h(\p)$. This is a contradiction to $\p = \arg\max_{x\in \Delta_K}\{\langle \y,\x \rangle-h(\x)\}$. Therefore, it must be the case that whenever $y_i > y_j$, $p_i \geq p_j$.
\end{proof}

\subsection{The Dueling Lemmas and Their Proofs}

%The proof of the theorem follows from Lemma \ref{lm:inductive_argument} and \ref{lm:mwu-nonconvergence}. Given the condition that $c \geq 3K^2$, we know $\rho = c$, so in this proof we will directly use $c$ as the normalization factor. 

As a high level, our proof leverage the above ``order-preserving'' property of mirror maps to prove, via a complex induction argument,  that if both players have significant probabilities to play the first $n$ actions within time $T_n$, then within time $(1+\frac{2c}{3K^2})T_k$, both players must also have significant amount of probabilities to play the first $n+1$ actions. This is enabled by the following ``dueling lemmas'', which reveal the intrinsic difficulty of using DA algorithms for iterated dominance elimination.

Intuitively, we w.o.l.g. show that for player $B$, any DA algorithm will have constant probability to play actions from $1,2,\cdots, n$ within $(1+\frac{2c}{3K^2})^{n-1}$ rounds, yielding the exponential-time convergence of DA algorithms for large $c$. The key challenge in this proof is the inter-agent utility externalities which makes the analysis of any player's utility depend on the other player's strategy, and vice versa. Our proof uses an induction argument. 

\begin{lemma}\label{lm:inductive_argument}
For any $1\leq n\leq K-2$, if there exists $T_n\geq 1$ such that 
\begin{equation}\label{eq:inductive_hypo}
    \sum_{i=1}^n p_{B,i}(t) \geq \frac{1}{K-n+1},\forall t\leq T_n, %\, \,  \sum_{i=1}^{n+1} p_{A,i}(t) \geq \frac{1}{K-n}, \, \, \forall t\leq T_n,
\end{equation}
then for  $T_{n+1}=(1+\frac{2c}{3K^2})T_n$ we will have 
\begin{equation}\label{eq:inductive_argument}
    \sum_{i=1}^{n+1} p_{B,i}(t) \geq \frac{1}{K-n},  \forall t\leq T_{n+1}. %\, \, \sum_{i=1}^{n+2} p_{A,i}(t) \geq \frac{1}{K-n-1}, \, \,  \forall t\leq T_{n+1}.
\end{equation}
\end{lemma}

\begin{proof}
We prove the claim by induction. When $n=1$, we can verify that $T_1=1$ satisfies Eq \eqref{eq:inductive_hypo}: since both players start by taking actions uniformly at random, we have 
$$p_{B,1}(1)=\frac{1}{K}\geq \frac{1}{K-1+1}.$$ %p_{A,1}+p_{A,2}=\frac{2}{K}\geq \frac{1}{K-1}.$$

Suppose Eq \eqref{eq:inductive_hypo} holds for some $T_n \geq 0$, next we show the validity of Eq \eqref{eq:inductive_argument}. At each step $t\leq T_n$, using the fact that $\sum_{i=1}^n p_{B,i}(t) \geq \frac{1}{K-n+1}$ and $\frac{K}{c} \leq \frac{1}{3K}$, we have 
    \begin{align} \notag
        u_{A,i}(t)
        &\leq\sum_{j=1}^n p_{B,j}(t)\cdot(-1)+(1-\sum_{j=1}^n p_{B,j}(t))\cdot(\frac{K}{c}), \quad \forall i=n+2,\cdots,K. \\ \notag
        & \leq \frac{1}{K-n+1}\cdot(-1)+(1-\frac{1}{K-n+1})\cdot(\frac{K}{c}) \\ \notag
        & \leq -\frac{1}{K-n+1}+ \frac{K-n}{K-n+1}\cdot \frac{1}{3K} \\ \label{eq:nega_uait}
        & < -\frac{2}{3(K-n+1)} \leq -\frac{2}{3K}.
    \end{align} 

As a result, player A's cumulative rewards on action ${n+2,\cdots, K}$ at step $t=T_n+1$ can thus be upper bounded by
    \begin{align}\notag
        y_{A,i}(T_n+1)&= \sum_{t=1}^{T_n}\eta_t u_{A,i}(t) < -\frac{2\sum_{t=1}^{T_n} \eta_t}{3K}, i=n+2,\cdots,K.
    \end{align}
    
    Then for $T_{n+1}=(1+\frac{2c}{3K^2})\cdot T_n$ and any $t\leq T_{n+1}$,  we have 
    \begin{align} \notag
        y_{A,i}(t) &= y_{A,i}(T_n+1) + \sum_{s=T_n+1}^{t-1}\eta_t u_{A,i}(s)  \\\notag 
        &<-\frac{2\sum_{t=1}^{T_n} \eta_t}{3K}+\frac{K}{c}\cdot \eta_{T_n+1}\cdot \frac{2c}{3K^2}\cdot T_n  \\ \label{eq:yait<0} 
        &\leq -\frac{2\sum_{t=1}^{T_n} (\eta_t-\eta_{T_n+1})}{3K}\leq 0, \forall i=n+2,\cdots,K.
    \end{align}
    
    Also note that $y_{A,1}(t)\geq 0, \forall t>0$, we thus conclude that $y_{A,i}(t)<y_{A,1}(t)$ for any $i\geq n+2$ and $t\leq T_{n+1}$. Applying Lemma \ref{lm:mono_Q}, we obtain $p_{A,i}(t)\leq p_{A,1}(t)$ and as a result, 
    \begin{align}\notag
        K-n-1 &\geq (K-n-1) \cdot [p_{A,1}(t) + \sum_{i=n+2}^{K} p_{A,i}(t)] \\ \notag
          & \geq \sum_{i=n+2}^{K} p_{A,i}(t) + (K-n-1)\cdot [\sum_{i=n+2}^{K} p_{A,i}(t)] \\ \label{eq:85}
          & = (K-n)[\sum_{i=n+2}^{K} p_{A,i}(t)],
    \end{align}
    which implies $\sum_{i=n+2}^{K} p_{A,i}(t)\leq \frac{K-n-1}{K-n}$ and thus
    \begin{equation}\label{eq:pa1kn1}
        \sum_{i=1}^{n+1} p_{A,i}(t)\geq \frac{1}{K-n}, \forall t\leq T_{n+1}.
    \end{equation}
    
    Now consider player B. Following the same logic as Eq \eqref{eq:nega_uait} and utilizing Eq \eqref{eq:pa1kn1}, we have 
    
    \begin{align*}
        u_{B,j}(t)
        &\leq\sum_{i=1}^{n+1} p_{A,i}(t)\cdot(-1)+(1-\sum_{i=1}^{n+1} p_{A,i}(t))\cdot(\frac{K}{c}) \\ 
        & \leq \frac{1}{K-n}\cdot(-1)+(1-\frac{1}{K-n})\cdot(\frac{K}{c}) \\ 
        & \leq -\frac{1}{K-n}+ \frac{K-n-1}{K-n}\cdot \frac{1}{3K} \\ 
        & < -\frac{2}{3(K-n)} \leq -\frac{2}{3K}, \forall n+2\leq j\leq K, t\leq T_{n+1}.
    \end{align*} 
    
    Hence, we similarly conclude that $y_{B,j}(t)<0\leq y_{B,1}(t)$ for any $j\geq n+2$ and $t\leq T_{n+1}$. Applying Lemma \ref{lm:mono_Q} yields $p_{B,j}(t)\leq p_{B,1}(t)$, and then we similarly follow Eq \eqref{eq:85} to obtain $\sum_{j=n+2}^{K} p_{B,j}(t)\leq \frac{K-n-1}{K-n}$ and thus
    \begin{equation}\label{eq:pb1kn1}
        \sum_{j=1}^{n+1} p_{B,j}(t)\geq \frac{1}{K-n}, \forall t\leq T_{n+1},
    \end{equation}
    which completes the proof.
\end{proof}

\subsection{Concluding the Proof. } 
Our final lemma leverages Lemma \ref{lm:inductive_argument} to shows that within $3^{K-2}$ time steps, any DA algorithm cannot play the unique equilibrium with large probability.   Note that since this particular setup has deterministic payoff and is in the perfect gradient feedback setup, Lemma \ref{lm:mwu-nonconvergence}  holds deterministically as well.  

\begin{lemma} \label{lm:mwu-nonconvergence} 
For any $K\geq 3 $, $c\geq 3K^2$ and any $t\leq 3^{K-2}$,
\begin{equation}\label{eq:nonconvergence}
    p_{A,K}(t)+p_{B,K}(t)\leq \frac{3}{2}.
\end{equation}

\end{lemma}

\begin{proof}

Take $n=K-2$ in Lemma \ref{lm:inductive_argument}, we immediately obtain from Eq \eqref{eq:inductive_argument} that
$$\sum_{i=1}^{K-1} p_{B,i}(t) \geq \frac{1}{2}, \forall t\leq T_{K-1},$$ 
where $T_{K-1}=(1+\frac{2c}{3K^2})^{K-2}\geq 3^{K-2}$. Therefore,
\begin{equation}\label{eq:final_1}
    p_{A,K}(t)+p_{B,K}(t)\leq 1+\frac{1}{2}=\frac{3}{2}, \forall t\leq 3^{K-2}.
\end{equation}

\end{proof}

Since $(K,K)$ is the unique NE of this game, Eq \eqref{eq:nonconvergence} implies that the probability that at least one of the agents is not playing the equilibrium is at least $\max \{ 1- p_{A,K}(t), 1- p_{B,K}(t) \} \geq \frac{ 1- p_{A,K}(t) + 1- p_{B,K}(t)}{2} \geq 1/4$. For example, if we take $c=3K^2$, Lemma \ref{lm:mwu-nonconvergence} tells us that DA cannot converge to the unique NE $(K,K)$ within the first $3^{K-2}$ iterations and thus implies an exponential convergence rate or even non-convergence. Also, a larger value of $c$ would further slow down the convergence rate.
